# Supplementary material for: An Emergent Space for Distributed Data with Hidden Internal Order through Manifold Learning
Source: arXiv:1708.05406 ancillary file (2018-12-06)
Supplement: Supplementary file 1 [file supplement.pdf]

# Supplemental Material

Felix P. Kemeth*[1, 2], Sindre W. Haugland*[1, 2], Felix Dietrich[3, 4], Tom Bertalan[5], Kevin Höhlein[1], Qianxiao Li[6], Erik M. Bollt[7], Ronen Talmon[8], Katharina Krischer[1], and Ioannis G. Kevrekidis[2, 3, 4]

[1] *Physik-Department, Nonequilibrium Chemical Physics, Technische Universität München, James-Franck-Str. 1, D-85748 Garching, Germany*
[2] *Institute for Advanced Study - Technische Universität München, Lichtenbergstr. 2a, D-85748 Garching, Germany*
[3] *The Department of Chemical and Biological Engineering - Princeton University, Princeton, NJ 08544, USA*
[4] *Department of Chemical and Biomolecular Engineering, Department of Applied Mathematics and Statistics, Johns Hopkins University and JHMI*
[5] *Department of Mechanical Engineering - MIT, Cambridge, MA 02139, USA*
[6] *Institute of High Performance Computing, 1 Fusionopolis Way, #16-16 Connexis North, Singapore 138632, Singapore*
[7] *Department of Mathematics, and Department of Electrical and Computer Engineering, Clarkson Center for Complex Systems Science, Clarkson University, Potsdam, NY 13699-5815, USA*
[8] *Department of Electrical Engineering - Technion - Israel Institute of Technology, Technion City, Haifa, Israel 32000*

## Figures 1 and 2 in the paper: Spatiotemporal intermittency in the complex Ginzburg-Landau equation

The complex Ginzburg-Landau equation (CGLE) in a re-scaled form reads

$$\partial_t W = W + (1 + ic_1)\nabla^2 W - (1 + ic_2)|W|^2 W,$$

with real parameters $c_1$ and $c_2$. The parameter values leading to our spatiotemporal intermittency [1] are $c_1 = 0$ and $c_2 = -3$. The equation is integrated using a pseudo-spectral integration method with exponential time-stepping [2] and fixed time step $dt = 0.05$. The system sizes considered are $L = 100$ with $N = 512$ grid points for one-dimensional simulations (Fig. 2) and $L_x = L_y = 40$ with $N_x = N_y = 64$ grid points for two-dimensional simulations (Fig. 3). The solution in both cases is sampled as $T = 1000$ snapshots between $t_0 = 500$ and $t_1 = 700$ time units. For the two-dimensional system, a kernel scale of $\epsilon = e^2 \approx 4.0 \cdot 10^{-3} D_{\text{max}}^2$ is chosen.

Fig. 1 in the paper discussed the spatial reconstruction of the solution from temporal observations. In that case, our data points consisted of 512 time series of length 1000 each. Fig. 1 below supports the claim made in the paper, that the same data-driven approach is also able to accomplish a temporal reconstruction of the solution from spatial observations. Here, the data points consisted of 1000 spatial snapshots of length 512. Clearly, the first diffusion maps component is now one-to-one with physical time, and the panels of the figure echo the ones of Fig. 2 in the paper.

*These authors contributed equally to this work.

©2018 IEEE  doi: 10.1109/ACCESS.2018.2882777

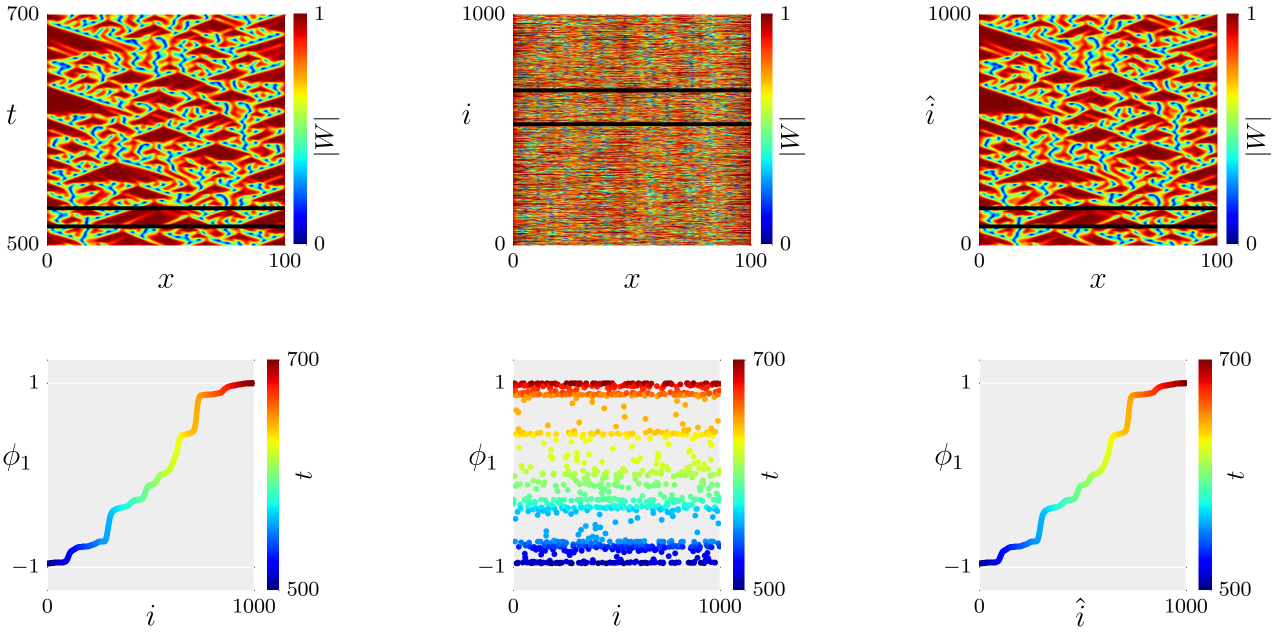


Figure 1: Reconstruction of the temporal arrangement of the one-dimensional spatiotemporal intermittency in the CGLE following the spatial reconstruction, Fig. 1 in the paper.

# Figure 3 in the paper: Heterogeneous Chung-Lu type network of pre-Bötzinger neurons

As a toy example for complex dynamics without an obvious physical space, we consider an ensemble of 1024 neurons, a caricature of the pre-Bötzinger complex [3–5],

$$\begin{aligned} C\frac{dV_i}{dt} &= -g_{\text{Na}} m\left(V_i\right) h_i\left(V_i - V_{\text{Na}}\right) - g_l\left(V_i - V_l\right) \\ &\quad + I^i_{\text{syn}} + I^i_{\text{app}} \\ \frac{dh_i}{dt} &= \frac{h_\infty\left(V_i\right) - h_i}{\tau\left(V_i\right)}. \end{aligned}$$

with the coupling

$$I^i_{\text{syn}} = \frac{g_{\text{syn}}\left(V_{\text{syn}} - V_i\right)}{N} \sum_{j=1}^{N} A_{ij} s\left(V_j\right).$$

Here

$$\begin{aligned} m\left(V\right) &= \left(1 + \exp\left(-\left(V + 37\right)/6\right)\right)^{-1}, \\ h_\infty\left(V\right) &= \left(1 + \exp\left(\left(V + 44\right)/6\right)\right)^{-1}, \\ \tau\left(V\right) &= \left(\epsilon \cosh\left(\left(V + 40\right)/5\right)\right)^{-1}, \\ s\left(V\right) &= \left(1 + \exp\left(-\left(V + 40\right)/5\right)\right)^{-1} \end{aligned}$$

are nonlinear functions, whereas $C = 0.21$, $g_{Na} = 2.8$, $g_l = 2.4$, $g_{\text{syn}} = 0.3$, $V_{\text{syn}} = 0$, $V_{\text{Na}} = 50$, $V_l = -65$ and $\epsilon = 0.1$ are constants. As in previous studies [5], we take the intrinsic kinetic

parameter $I_{app}^i$ to vary across the ensemble ($I_{app}^i = 22 + 2\omega_i$, where $\omega_i$ is drawn from a uniform distribution on $[-1, 1]$), making the network kinetically heterogeneous.

We connect the neurons in the form of a Chung-Lu type network [6], where the network topology is given by a symmetric adjacency matrix $\mathbf{A}$. The entries $A_{ij}$ are 1 if there is a coupling between oscillators $i$ and $j$, and 0 otherwise. The algorithm for the creation of the $A_{ij}$ uses a sequence of weights $w_i$ for each oscillator $i$, defined as

$$w_i = pN(i/N)^r \quad , \quad i = 1, 2, ..., N$$

with parameters $p = 0.80$ and $r = 0.40$. From these weights, the entries $P_{ij}$ of a matrix $\mathbf{P}$ of connection probabilities are defined as

$$P_{ij} = P_{ji} = \min\left(\frac{w_i w_j}{\sum_k w_k}, 1\right) .$$

The matrix is then mirrored along the diagonal, and all diagonal entries are set to zero to avoid self-loops. As initial conditions, $V = -60.0$ and $h = 0.0$ are taken for all oscillators. We simulated our realization of a Chung-Lu network of $N = 1024$ oscillators, using LSODE [7, 8]. The time series observations from each neuron were taken between $t_0 = 20$ and $t_1 = 40$ in the form of $T = 2001$ time steps.

# Figure 4 in the paper: Type-II chimera in the modified complex Ginzburg-Landau equation

The modified complex Ginzburg-Landau equation (MCGLE), that is, the CGLE with nonlinear global coupling, is described by

$$\begin{aligned}\partial_t W \; = \; & -i\nu W + (1 + ic_1)\nabla^2 W \\ & - (1 + i\nu)(\langle W \rangle - W) \\ & + (1 + ic_2)\left(\langle |W|^2 W \rangle - |W|^2 W\right)\end{aligned}$$

with $\langle \ldots \rangle$ denoting spatial averages. It has the property that for the spatially uniform mode,

$$\partial_t \langle W \rangle = -i\nu \langle W \rangle \;\Rightarrow\; \langle W \rangle = \eta e^{-i\nu t}$$

holds. Thus, the mean $\langle W \rangle$ is confined to harmonic motion with frequency $\nu$ and amplitude $\eta$ [9]. This system is known to exhibit type-II chimeras for $c_1 = 0.2$, $c_2 = -0.63$, $\nu = 0.1$ and $\eta = 0.65$, starting from random initial conditions. Here, a system size of $L = 100$ with periodic boundaries and $N = 4096$ grid points is considered. For integration, a pseudo-spectral method with exponential time-stepping [2] and fixed time step of $dt = 0.01$ was used. The data was sampled between $t_0 = 5000$ and $t_1 = 6000$ at $T = 4000$ snapshots. Data mining for different values of the kernel scale parameter $\epsilon$ was performed on 4096 time series of length 4000 each.

# Figure 5 in the paper: Modulated traveling waves in the 1-D Kuramoto-Sivashinsky equation

The Kuramoto-Sivashinsky equation in one spatial dimension reads

$$\partial_t u + \alpha\left(u\partial_x u + \partial_{xx} u\right) + 4\partial_{xxxx} u = 0$$

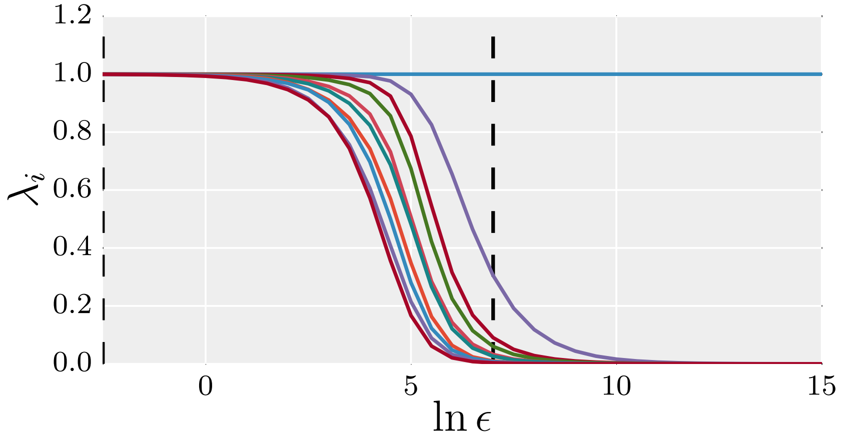


Figure 2: The dominant ten eigenvalues of the eigenvalue spectrum obtained from the diffusion matrix for different values of the kernel parameter $\epsilon$.

with the real variable $u = u(x, t)$ and a single real parameter $\alpha$. For system size $L = 2\pi$, with periodic boundary conditions, and $\alpha = 53.3$, the equation is known to exhibit stable modulated traveling waves [10]. Using $N = 100$ spatial grid points in a finite-difference discretization, we numerically integrate the Kuramoto-Sivashinsky equation using lsode [7, 8] with time step $dt = 0.001$ and sample the data between $t_0 = 1$ and $t_1 = 1.25$ as $T = 500$ snapshots. We are confident that our simulation has reasonably converged on the attractor by $t_0 = 1$, so that our 100 time series of length 400 are representative of it. For completeness, we note here that one period of the modulation contains $\approx 56$ discrete snapshots and the "period" of traveling in the spatially periodic domain is known to consist of $\approx 250$ snapshots.

# Figure 6 in the paper (Gauge-invariant diffusion maps), and the Koopman operator

We illustrate the capability of performing gauge-invariant diffusion map computations on a simple two-dimensional nonlinear dynamical system possessing a stable limit cycle in its deterministic form, yet slightly perturbed by low-amplitude white noise. We start by recording the evolution of its state. Separately, we record observations of this evolution through a known "observation function" that transforms this state nonlinearly (and invertibly). In the original system, for short time intervals, the white noise causes states initialized at a single point $(r, \theta)$ to spread out to a normal distribution. In the observed system (here, observed through the observation function $T(r, \theta) = [(r^2)\cos(\theta)/2, \sqrt{r}\sin(\theta)])$, the normal distribution is transformed into an ellipsoid shape, with axes corresponding to the eigenvectors of the noise covariance matrix $C = J(r, \theta)J(r, \theta)^T$– where $J$ is the Jacobian of the transformation function $T$. Thus, observing several brief bursts of (stochastic) simulation initialized at a particular state-space point through $T$ allows us to estimate the covariance matrix $C$ numerically. The pseudo-inverse of this matrix is used to compute the Mahalanobis-like distance between two data points $x, y$ (see [11, 12]):

$$d(x, y)^2 = 1/2(x - y)^T (C(x) + C(y))^{-1}(x - y).$$

The "gauge invariant" diffusion maps, based on using this Mahalanobis-like distance for each of the two observations, visibly yields (and can be shown to successfully approximate) *the same*

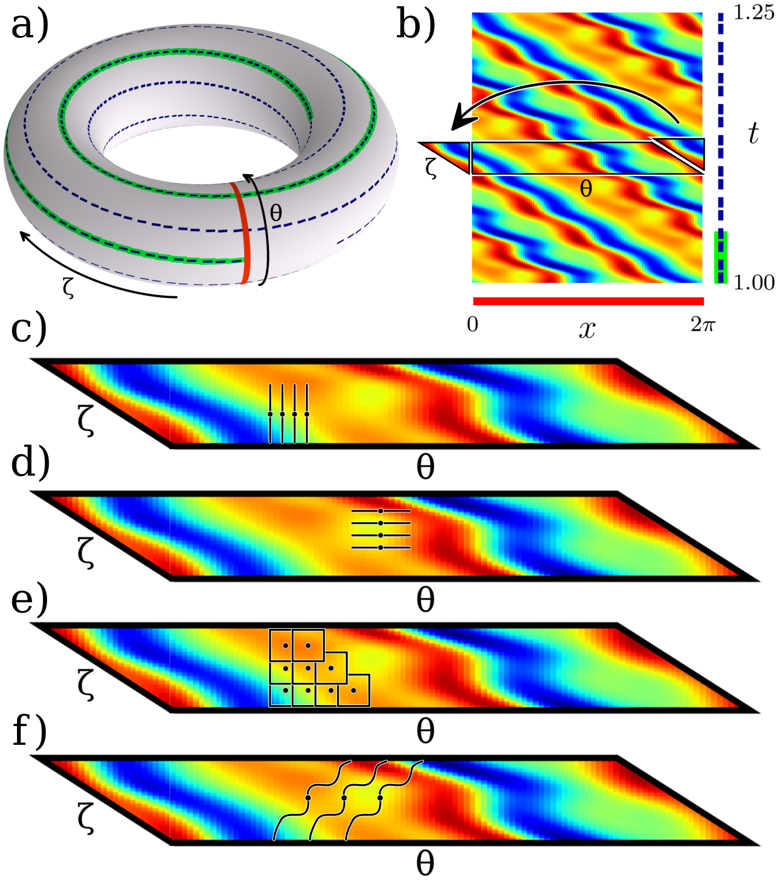


Figure 3: (a) In a system exhibiting the dynamics of a modulated traveling wave, the state of any point in space and time can be described by its phase with respect to the modulation ($\zeta$) and traveling wave ($\theta$), respectively. Together, these two phases span the surface of a torus. (b) The data set from the Kuramoto-Sivashinsky equation treated in the paper section on observing an attractor is an example of such dynamics, containing the "minimal parallelogram" of the unfolded torus several times over.. (c-f) The points in this minimal parallelogram can be observed in several different ways, either as time strings (c), space strings (d), space-time patches (e) or through the trajectories of active observers (f) that travel with their own, known speeds along the torus surface.

embedding (Fig. 6 in the paper) modulo an orthogonal transformation. Clearly, the (invertible) mapping of any trajectory of the original system to the corresponding trajectory of the transformed (diffeomorphic) one provides a systematic way of matching the two systems, mapping one to the other, and even fusing observations from both of them (see e.g. [13]). This transformation is encoded in the eigenvectors of the gauge invariant diffusion map matrix (that approximate the eigenfunctions of the Laplace-Beltrami operator on the data manifold).

We now discuss an alternative approach to the construction of data-driven conjugacies: one using the Koopman operator framework [14], which also employs a spectral representation. For a discrete dynamical system $x_{k+1} = f(x_k)$, $x \in \mathbb{R}^n$, the Koopman operator $\mathcal{K}$ acts linearly on a space of complex-valued observables $h : \mathbb{R}^n \to \mathbb{C}$. Specifically, for any given observable $h$, $(\mathcal{K}h)(x) = (h \circ f)(x)$. This property also gives it the name *composition operator*. Indeed, exploring the numerically obtained spectra of the Koopman operator (see [15]) for each of the two deterministic systems, we can also find matching eigenvalues and eigenfunctions, analogous to

the gauge-invariant diffusion map case. If $\psi$ is a Koopman eigenfunction of the original system associated to the eigenvalue $\lambda$, $\psi = \hat{\psi} \circ T$ defines an eigenfunction $\hat{\psi}$ of the observed system associated to the same eigenvalue. This relation can be used to approximate the function $T$ if enough pairs of eigenfunctions $(\psi, \hat{\psi})$ are given [16]. There are already numerous algorithms available to approximate Koopman eigenfunctions, such as EDMD [17] in the general case and Fourier- or Laplace-Averaging for limit cycle systems [18]. Here we use the Fourier average defined as $f_\omega(x) = \lim_{N\to\infty} \frac{1}{N} \sum_{k=0}^{N} (h \circ f^k)(x) \exp(-i\omega k)$, where $\omega$ is the period of the limit cycle and $f$ is a generic observable of the system state. The resulting function $f_\omega : \mathbb{R}^n \to \mathbb{C}$ is an eigenfunction of the Koopman operator [18], such that $\mathcal{K} f_\omega = \exp(i\omega) f_\omega$. For continuous systems $\dot{x} = \frac{d}{dt} S^t|_{t=0}(x)$, the Fourier average is defined as $f_\omega(x) = \lim_{t\to\infty} \frac{1}{t} \int_0^t (h \circ S^{t'})(x) \exp(-i\omega t') dt'$. We compute the Fourier averages with the observable $h(x) = x_1 + x_2$ similar to [18], where $x_1, x_2$ are the Cartesian coordinates of the system. The (complex-valued) eigenfunction $f_\omega$ then defines the geometry in the Koopman eigenfunction space (see Fig. 4). The geometry in this space allows us to learn the (approximate) transformation function through a standard optimization formulation, in our case, a two-hidden-layer neural network. In particular, we solve $\min_{T:\mathbb{R}^2\to\mathbb{R}^2} \|\psi - \phi \circ T\|^2_{L^2(\mathbb{R}^2)}$ by parameterizing $T$ as a two-layer feed-forward neural network with 10 hidden units, i.e. $T(\mathbf{x}) = V\sigma(W\mathbf{x} + \mathbf{b}) + \mathbf{c}$, where $W \in \mathbb{R}^{10\times 2}$, $\mathbf{b} \in \mathbb{R}^{10}$, $V \in \mathbb{R}^{2\times 10}$, $\mathbf{c} \in \mathbb{R}^2$, and $\sigma$ is a sigmoid point-wise nonlinearity $\sigma(\mathbf{x})_i = 1/(1 + e^{-x_i})$. We solve the minimization by standard stochastic gradient descent, with samples uniformly drawn in the set $|\mathbf{x}|^2 < 1.4$. The approximation by a neural network is scalable to larger problems because it circumvents the "curse of dimensionality" associated with the usual function approximation via linear combination of basis functions. Now, the transformation function is embodied in the neural network.

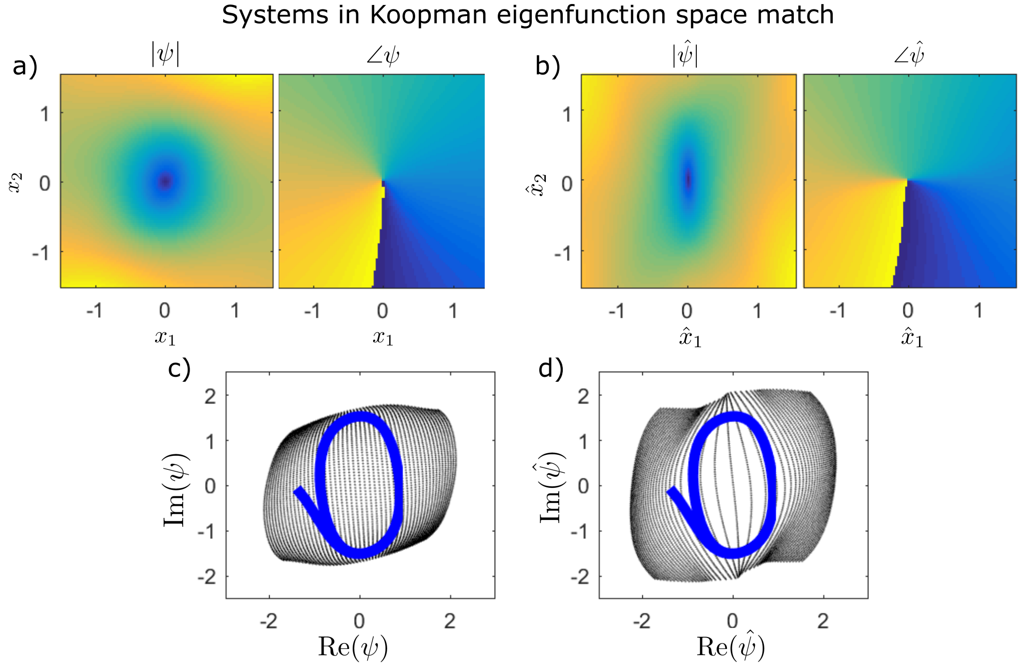


Figure 4: Eigenfunctions of the Koopman operator are computed by Fourier average, and interpolated with a neural network, for the original system (a), and the transformed system (b). Drawn in the real and complex parts of the eigenfunction, the trajectories of both systems match (plots c,d). The black dots in plots (c,d) visualize the transformation of the plane $[-1, 1]^2$ into the Koopman eigenfunction space.

# Video 1: Type-I chimera state in the 2-d globally coupled complex Ginzburg-Landau equation

We integrate the complex Ginzburg-Landau equation with nonlinear global coupling (as described above) for parameters $c_1 = 0.2$, $c_2 = 0.61$, $\nu = 1.5$ and $\eta = 1.0$ on a two-dimensional spatial domain of size $750 \times 750$ and fixed time step $dt = 0.01$. The data is sampled from $t_0 = 1900$ to $t_1 = 2000$ as $T = 500$ snapshots. For these parameters, the system exhibits a so-called type-I chimera state, for which the absolute value $|W|$ of the complex system variable is used as $z$-axis in the right part of video 1.

Following earlier works on chimera states [19], we apply a scaled version of the discrete Laplacian to the data,

$$\begin{aligned}\mathbf{D}f(x,y,t) \;=\;& f\left(x+\Delta x,y,t\right)+f\left(x-\Delta x,y,t\right)\\ &+f\left(x,y+\Delta y,t\right)+f\left(x,y-\Delta y,t\right)\\ &-4f\left(x,t\right)\,.\end{aligned}$$

Creating a histogram of these transformed data may reveal insightful features of different chimera states. In the left part of video 1, a two-dimensional histogram over the angle $\angle D$ of the complex-valued Laplacian and the absolute value $|W|$ of the complex system variable is shown.

A circular one-dimensional color scale is used to encode the individual bins of histogram. Every individual point in physical space (right part of the video) is then colored according to bin (and thus, the color) to which it corresponds. Special care is taken for the coherent regimes of the chimera state, as the value of $D$ vanishes there and the angle $\angle D$ becomes thus not well-defined. Accordingly, all points with amplitude $|W|$ larger 1 are given the same blueish-purple color.

# Video 2: 3-d histogram of the type-I chimera state

For the same data obtained in the previous section, a different representation is chosen in video 2. Here, a three-dimensional histogram is created over the absolute value $|W|$ of the complex system variable, and the real and imaginary parts of the discrete Laplacian $D$. The "height" of the bins in this histograms are encoded in the size and the color of the scattered points in the left part of the video. In addition, projections onto two-dimensional histograms are depicted in the three planes parallel to $(\mathrm{Re}D, \mathrm{Im}D)$, $(\mathrm{Re}D, |W|)$ and $(\mathrm{Im}D, |W|)$.

# Video 3: Type-I chimera state in a Stuart-Landau ensemble

Video 3 shows the data of a chimera state arising in an ensemble of $N = 10000$ Stuart-Landau oscillators, globally coupled as

$$\begin{aligned}\partial_t W =& -i\nu W-(1+i\nu)\left(\langle W\rangle_\Sigma - W\right)\\ &+(1+ic_2)\left(\langle |W|^2 W\rangle_\Sigma - |W|^2 W\right)\,,\end{aligned}$$

with $\langle W\rangle_\Sigma = 1/N \sum_i W_i$ and $\langle |W|^2 W\rangle_\Sigma = 1/N \sum_i |W_i|^2 W_i$ denoting ensemble averages. It has the property that for the spatially uniform mode, the relation

$$\partial_t \langle W\rangle = -i\nu\langle W\rangle \;\Rightarrow\; \langle W\rangle = \eta e^{-i\nu t}$$

holds. Thus, the mean $\langle W \rangle$ is confined to harmonic motion with frequency $\nu$ and amplitude $\eta$ [9].

The system is integrated using LSODE [7,8] with fixed time step $dt = 0.01$ at parameter values $c_2 = 0.58$, $\nu = 1.49$ and $\eta = 1.02$, and the data is sampled from $t_0 = 500$ to $t_1 = 525$ as $T = 500$ snapshots.

The real parts of the individual oscillators are depicted on the right, and a two-dimensional histogram over the real and imaginary parts of the complex system variable $W$ in a co-rotating frame, rotating with the frequency of the ensemble mean, $\nu$, on the left. Moreover, the individual bins of histogram are encoded with a circular one-dimensional color scale, corresponding to the angle $\angle W$. Every individual oscillator in the right part of the video is then colored according to the bin (and thus, the color) to which it corresponds.

# Video 4: Type-I chimera state in the 1-D globally coupled complex Ginzburg-Landau equation

This video illustrates the evolution of characteristics on an attractor: The temporal evolution of observables for fixed physical space (on the right) compared to how physical space "visits" different observable values as time passes (on the left).

In order to generate the data for video 4, we integrate the complex Ginzburg-Landau equation with nonlinear global coupling as described above, but on a one-dimensional spatial domain of length $L = 1000$. The simulation is carried out for parameters $c_1 = 0.2$, $c_2 = 0.61$, $\nu = 1.5$ and $\eta = 1.0$ with a fixed time step $dt = 0.01$. The data is sampled from $t_0 = 2500$ to $t_1 = 2530$ as $T = 300$ snapshots. For these parameters, this system exhibits a so-called type-I chimera state, for which the real value of the complex system $W$ variable is shown as a function of space in the right part of video 4.

In order to create the two other parts of the video, we apply a scaled version of the 1-D discrete gradient, defined as

$$\mathbf{d}_{\mathrm{x}} f(x,t) \ = \ f\left(x+\Delta x, t\right) - f\left(x-\Delta x, t\right) \, .$$

In the left part of video 4, a two-dimensional histogram over the real part $\mathrm{Re} d_{\mathrm{x}}$ of the complex-valued gradient and the absolute value $|W|$ of the complex system variable is shown. A projection of this histogram, showing all non-empty bins, is shown in the form of several black lines on the plane parallel to $(\mathrm{Re} d_{\mathrm{x}}, |W|)$ (below the histogram itself). The resulting long, "snake-like" self-intersecting black curve is parametrized by physical space - its evolution shows which observable values are realized (are "visited" by physical space) as time evolves.

In the middle part of the video, the last 15 such projections are plotted above each other, with the newest projection shown at the top, and every projection being moved one step downward every frame increment of the video.

Finally, a circular one-dimensional color scale is used to encode the individual bins of the histogram in the left part of the video. Every individual points in physical space (right part of the video) is then colored according to the bin (and thus, the color) to which it corresponds [cite vid_4.avi].

All figures are generated using matplotlib [20].

# References


[1] B.I. Shraiman, A. Pumir, W. van Saarloos, P.C. Hohenberg, H. Chaté, and M. Holen. Spatiotemporal chaos in the one-dimensional complex Ginzburg-Landau equation. *Physica D: Nonlinear Phenomena*, 57(3):241–248, 1992.

[2] S.M. Cox and P.C. Matthews. Exponential Time Differencing for Stiff Systems. *Journal of Computational Physics*, 176(2):430–455, mar 2002.

[3] Jonathan Rubin and David Terman. Synchronized activity and loss of synchrony among heterogeneous conditional oscillators. *SIAM Journal on Applied Dynamical Systems*, 1(1):146–174, 2002.

[4] Carlo R. Laing, Yu Zou, Ben Smith, and Ioannis G. Kevrekidis. Managing heterogeneity in the study of neural oscillator dynamics. *The Journal of Mathematical Neuroscience*, 2(1):1–22, 2012.

[5] M. Choi, T. Bertalan, C.R. Laing, and I.G. Kevrekidis. Dimension reduction in heterogeneous neural networks: Generalized Polynomial Chaos (gPC) and ANalysis-Of-VAriance (ANOVA). *The European Physical Journal Special Topics*, 225(6):1165–1180, Sep 2016.

[6] Carlo R. Laing, Karthikeyan Rajendran, and Ioannis G. Kevrekidis. Chimeras in random non-complete networks of phase oscillators. *Chaos*, 22(1):013132, 2012.

[7] A.C. Hindmarsh. *LSODE. Ordinary Differential Equation System Solver.* Dec 1986.

[8] K Radhakrishnan and A C Hindmarsh. *Description and use of LSODE, the Livemore Solver for Ordinary Differential Equations.* Dec 1993.

[9] Lennart Schmidt, Konrad Schönleber, Katharina Krischer, and Vladimir García-Morales. Coexistence of synchrony and incoherence in oscillatory media under nonlinear global coupling. *Chaos*, 24(1), 2014.

[10] H S Brown and I G Kevrekidis. Modulated traveling waves for the Kuramoto-Sivashinsky equation. In *Pattern Formation: Symmetry Methods and Applications (Fields Institute Communication)*, volume 5, Providence, RI, 1996. American Mathematical Society.

[11] Boaz Nadler, Stéphane Lafon, Ronald R. Coifman, and Ioannis G. Kevrekidis. Diffusion maps, spectral clustering and reaction coordinates of dynamical systems. *Applied and Computational Harmonic Analysis*, 21(1):113–127, 7 2006.

[12] Amit Singer and Ronald R. Coifman. Non-linear independent component analysis with diffusion maps. *Applied and Computational Harmonic Analysis*, 25(2):226–239, 2008.

[13] Carmeline J. Dsilva, Ronen Talmon, Neta Rabin, Ronald R. Coifman, and Ioannis G. Kevrekidis. Nonlinear intrinsic variables and state reconstruction in multiscale simulations. *The Journal of Chemical Physics*, 139(18):184109, 2013.

[14] Bernard Osgood Koopman. Hamiltonian systems and transformation in Hilbert space. *Proceedings of the National Academy of Sciences of the USA*, 17(5):315–318, 1931.

[15] Marko Budišić, Ryan Mohr, and Igor Mezić. Applied koopmanism. *Chaos*, 22:047510, 2016.

[16] Erik M. Bollt, Qianxiao Li, Felix Dietrich, and Ioannis Kevrekidis. On matching, and even rectifying, dynamical systems through Koopman operator eigenfunctions. *SIAM Journal on Applied Dynamical Systems*, 17(2):1925–1960, jan 2018.

[17] Matthew O. Williams, Ioannis G. Kevrekidis, and Clarence W. Rowley. A data-driven approximation of the koopman operator: Extending dynamic mode decomposition. *Journal of Nonlinear Science*, 25(6):1307–1346, 2015.

[18] A. Mauroy, I. Mezić, and J. Moehlis. Isostables, isochrons, and koopman spectrum for the action–angle representation of stable fixed point dynamics. *Physica D: Nonlinear Phenomena*, 261:19–30, 2013.

[19] Felix P. Kemeth, Sindre W. Haugland, Lennart Schmidt, Ioannis G. Kevrekidis, and Katharina Krischer. A classification scheme for chimera states. *Chaos*, 26(9):094815, 2016.

[20] J. D. Hunter. Matplotlib: A 2d graphics environment. *Computing In Science & Engineering*, 9(3):90–95, 2007.
